# Supplementary material for: Label-Efficient Online Continual Object Detection in Streaming Video
Source: arXiv:2206.00309 source file (2023-08-23)
Supplement: Supplementary file 1 [file suppl_without_replay.tex]

% Please add the following required packages to your document preamble:
% \usepackage{multirow}
% \usepackage{graphicx}
\begin{table}[h!]
\centering
\resizebox{0.48\textwidth}{!}{%
\begin{tabular}{ccccc}
\hline
\multicolumn{1}{l}{} &
  Annotation Cost &
  FAP ($\uparrow$) &
  CAP ($\uparrow$) &
  F ($\downarrow$) \\ \hline
\multirow{5}{*}{iCaRL(our impl.) w/o replay} &
  100\% &
  7.70 &
  8.03 &
  0.72 \\
 & 50\%   & 6.87 & 7.19  & 0.97  \\
 & 25\%   & 6.02 & 5.41  & 1.13  \\
 & 12.5\% & 4.56 & 5.09  & -0.02 \\
 & 6.25\% & 3.43 & 3.25  & -0.26 \\ \hline
\multirow{5}{*}{\begin{tabular}[c]{@{}c@{}}Efficient-CLS w/o replay\\ (EMA only)\end{tabular}} &
  100\% &
  9.79 &
  14.09 &
  -2.13 \\
 & 50\%   & 8.63 & 12.15 & -1.54 \\
 & 25\%   & 7.54 & 9.89  & -1.82 \\
 & 12.5\% & 5.95 & 8.00  & -1.45 \\
 & 6.25\% & 4.84 & 6.29  & -1.32 \\ \hline
\multirow{5}{*}{\begin{tabular}[c]{@{}c@{}}Efficient-CLS w/o replay\\ (EMA+Pseudo-labeling)\end{tabular}} &
  100\% &
  9.79 &
  14.09 &
  -2.13 \\
 & 50\%   & 8.45 & 11.93 & -1.98 \\
 & 25\%   & 6.36 & 8.53  & -1.39 \\
 & 12.5\% & 4.52 & 5.80  & -0.98 \\
 & 6.25\% & 2.63 & 2.97  & -0.17 \\ \hline
\end{tabular}%
}
\vspace{2mm}
\caption{\textbf{Performance of Efficient-CLS and other state-of-the-art methods without episodic replay on OAK dataset.}}
\label{stab:without_replay}
\end{table}
